# Supplementary material for: Strings of droplets propelled by coherent waves
Source: arXiv:1504.00484 ancillary file (2015-04-02)
Supplement: Supplementary file 1 [file Modele.pdf]

# Supplementary information - Model for a string of walkers

The motion of a walker on the liquid surface originates from the coupling between the droplet and the waves emitted at each impacts. An empirical model has been proposed by Fort and coworkers in [1] to describe the walking behavior taking advantage of the stroboscopic nature of the dynamics. One has

$$u_{n+1} - u_n = -\gamma u_n - C_0 \left.\frac{\partial \zeta}{\partial s}\right|_{n+1}. \tag{1}$$

In this expression, $u$ is the walker speed along the $s$-direction, the subscript $n$ refers to the $n$th impact and the coefficient $C_0$ represents the coupling between the walker and its own wave-field $\zeta(s,t)$. Besides the wave-coupling term, a friction term has been added to take account of the dissipation of energy during impacts, with $\gamma$ being the viscous-like coefficient. One can generalize this model to $N$ droplets bouncing on the bath by considering the linear superposition of all produced wave-field.

$$u^i_{n+1} - u^i_n = -\gamma u^i_n - C_0 \left.\frac{\partial \zeta^{ii}}{\partial s}\right|_{n+1} - C_1 \sum_{j\neq i} \left.\frac{\partial \zeta^{ij}}{\partial s}\right|_{n+1}. \tag{2}$$

The superscript of the speed refers to the $i$th walker on the surface and the superscripts of the wave-field denote the interaction of walker $i$ with the wave-field arising from walker $j$. For this term, a coupling coefficient $C_1$ is considered and may be different from $C_0$. This difference comes from the dissipation of energy outside the channel. The waves emitted by a walker in the channel reads

$$\zeta^{ij}(s^i,t) = \zeta_0 \cos\left(k_F(s^i(t) - s^j_{imp})\right) \exp\left(-\frac{s^i(t) - s^j_{imp}}{\delta}\right) \exp\left(-\frac{t - t^j_{imp}}{\tau}\right), \tag{3}$$

where $k_F$ is the Faraday wave number and $s^j_{imp}$ and $t^j_{imp}$ are the impact position and time respectively. The viscosity of the bath has been taken into account with the exponential factor $\exp(-(s^i(t) - s^j_{imp})/\delta)$ where $\delta$ is some viscous length. The so-called *memory* of the walker has been considered with the factor $\exp(-(t-t^j_{imp})/\tau)$ where $\tau$ is the memory time. In the case of several impacts, the wave-fields have to be summed up over the whole trajectory leading to

$$\zeta^{ij}(s^i,t) = \zeta_0 \sum_{p=-\infty}^{n} \cos\left(k_F(s^i(t) - s^j_p)\right) \exp\left(-\frac{s^i(t) - s^j_p}{\delta}\right) \exp\left(-\frac{t - t^j_p}{\tau}\right). \tag{4}$$

It has been shown in [2] and [3] that, in the case of a 1D dynamics and in the low memory regime, the total wave field can be simplified by considering only the last impact with an equivalent amplitude $\zeta_{eq}$. One has

$$\zeta^{ij}(s^i,t) = \zeta_{eq} \cos\left(k_F(s^i(t) - s^j_{last})\right) \exp\left(-\frac{s^i(t) - s^j_{last}}{\delta}\right) \tag{5}$$

where $s^j_{last}$ and $t^j_{last}$ are the last impact position and time respectively. Knowing the total wave-field and assuming a stationary regime where $s^i_{n+1}(t) - s^i_n = u^i_n \tau_F$, one gets, in the particular case of two walkers :

$$\begin{aligned} u^1_n = &\frac{C_0}{\gamma}\left(\sin\left(k_F\tau_F u^1_n\right) + \frac{1}{k_F\delta}\cos(k_F\tau_F u^1_n)\right)\exp\left(-\frac{\tau_F u^1_n}{\delta}\right) \\ &\pm \frac{C_1}{\gamma}\left(\sin\left(k_F(\tau_F u^2_n + d)\right) + \frac{1}{k_F\delta}\cos(k_F(\tau_F u^2_n + d))\right)\exp\left(-\frac{\tau_F u^2_n + d}{\delta}\right), \end{aligned} \tag{6}$$

$$\begin{aligned} u^2_n = &\pm\frac{C_1}{\gamma}\left(\sin\left(k_F(\tau_F u^1_n - d)\right) - \frac{1}{k_F\delta}\cos(k_F(\tau_F u^1_n - d))\right)\exp\left(-\frac{d - \tau_F u^1_n}{\delta}\right) \\ &+ \frac{C_0}{\gamma}\left(\sin\left(k_F\tau_F u^2_n\right) + \frac{1}{k_F\delta}\cos(k_F\tau_F u^2_n)\right)\exp\left(-\frac{\tau_F u^2_n}{\delta}\right), \end{aligned} \tag{7}$$

where $\pm$ accounts for synchronized or anti-synchronized droplets and $d = s^1 - s^2$ is the interdistance between

the walkers. Assuming the same speed for both droplets ($u_n^1 = u_n^2 = v_2$) leads to the following conditions

$$\sin\left(k_F(\tau_F v_2 + d)\right) + \frac{1}{k_F\delta}\cos(k_F(\tau_F v_2 + d)) = \left(\sin\left(k_F(\tau_F v_2 - d)\right) - \frac{1}{k_F\delta}\cos(k_F(d - \tau_F v_2))\right)\exp\left(\frac{2\tau_F v_2}{\delta}\right), \quad (8)$$

$$v_2 = \frac{C_0}{\gamma}\left(\sin\left(k_F\tau_F v_2\right) + \frac{1}{k_F\delta}\cos(k_F\tau_F v_2)\right)\exp\left(-\frac{\tau_F v_2}{\delta}\right) \pm \frac{C_1}{\gamma}\left(\sin\left(k_F(\tau_F v_2 + d)\right) + \frac{1}{k_F\delta}\cos(k_F(\tau_F v_2 + d))\right)\exp\left(-\frac{\tau_F v_2 + d}{\delta}\right). \quad (9)$$

The first equation gives the distance quantification and the second one gives the speed of a pair of drops $v_2$. Because of the non-linearity of both equations, one needs to solve then by iteration. Taking initially $v_2 = v_1$, the speed of a single walker and $d = n\lambda_F/2$, the multiples of the half Faraday wave-length, leads to Fig? with coefficient $C_0/\gamma = 0.0282$, $C_1 = 0.05C_0$ and $\delta = 2.1\lambda_F$. Eqs.(8) and (9) converge to a solution after a tenth of iterations. The value of $\delta$ is close to the one encountered in models of walkers [3]. The value of $C_1$ compared to $C_0$ shows that only 5% of the wave emitted by walker $j$ acts on walker $i$. One can understand the decrease of $v_2$ as a function of $\delta$ because of the factor $\exp(-(\tau_F v_2 + d)/\delta)$ in Eq.(9). This behavior is due to the viscous properties of the bath that leads to an exponential damping of the waves. One can also rationalize a value of $v_2$ higher than $v_1$ by checking the values of $d$ and the synchronicity of the bounce. Those values are the ones that lead to constructive interference of the surface waves. Because the walker speed is directly proportional to the slope oh the waves, a higher amplitude leads to a faster motion.

In the case of $N$ droplets, one assumes that the quantified interdistance between the droplets are unchanged. Doing so, the speed $v_N$ of a chain of droplets is

$$v_N = \frac{C_0}{\gamma}\left(\sin\left(k_F\tau_F v_N\right) + \frac{1}{k_F\delta}\cos(k_F\tau_F v_N)\right)\exp\left(-\frac{\tau_F v_N}{\delta}\right) \pm \frac{C_1}{\gamma}\sum_{i=1}^{n}\left(\sin\left(k_F(\tau_F v_N + id)\right) + \frac{1}{k_F\delta}\cos(k_F(\tau_F v_N + id))\right)\exp\left(-\frac{\tau_F v_N + id}{\delta}\right). \quad (10)$$

The results of this equation is given on Fig.4 and reproduce the increase of the speed thanks to constructive interference.

We show that a model based on the superposition of all waves reproduces the observed experimental behavior. Thanks to constructive interferences, the coherent wave propels the string of droplets faster than single ones. Furthermore, as the distance between the walkers increases, the speed is reduced because of the viscous damping.

# References


[1] E. Fort, A. Eddi, A. Boudaoud, J. Moukhtar and Y. Couder, PNAS **107**, 17515 (2010).

[2] M. Labousse and S. Perrard, Phys. Rev. E **90**, 022913 (2014).

[3] C. Borghesi, J. Moukhtar, M. Labousse, A. Eddi, E. Fort and Y. Couder, Phys. Rev. E **90**, 063017 (2014).
